# Supplementary material for: Stationary ordered non-equilibrium states of long-range interacting systems
Source: arXiv:1705.05623 source file (2017-07-15)
Supplement: Supplementary file 1 [file SM_OQSS_FINAL_v3.pdf]

# Stationary ordered non-equilibrium states of long-range interacting systems: Supplemental Material

Michael Joyce[1], Jules Morand[2] and Pascal Viot[3]
[1] *Laboratoire de Physique Nucléaire et de Hautes Énergies, UPMC IN2P3 CNRS UMR 7585, Sorbonne Universités, 4, place Jussieu, 75252 Paris Cedex 05, France*
[2] *National Institute for Theoretical Physics (NITheP),Stellenbosch 7600, South Africa & Institute of Theoretical Physics, Department of Physics, Stellenbosch University, Stellenbosch 7600, South Africa and*
[3] *Laboratoire de Physique Théorique de la Matière Condensée, UPMC, CNRS UMR 7600, Sorbonne Universités, 4, place Jussieu, 75252 Paris Cedex 05, France*

## I. SIMULATION ALGORITHM

We consider the model of $N$ point particles interacting via an attractive pair potential $v(r) = gr^{\alpha}$ where $r$ is the distance between a pair of particles in one dimension, and $g$ the coupling constant which has the same sign as the exponent $\alpha$, to which the collision rules discussed in our article are applied when particles cross. For $\alpha < 1$ the force between two particles diverges when particles cross, and we thus adopt a regularised version, introducing a "smoothing scale" $\epsilon$ and taking $v(r) = g[r^2 + \epsilon^2]^{\alpha/2}$. For $\alpha = 1$ and $\alpha = 2$, the dynamics and collisions rules can be solved for exactly (up to the numerical round-off errors) by using an event-driven algorithm (see e.g. [1] and references therein) because the equations of motion between particle crossings can be solved for exactly. The specific results given in the figures of the article are for the case $\alpha = 1$ and have been obtained with such an algorithm. The generalisation of our findings to the range $\alpha \in [-1, 2]$ and the HMF model, which we detail further here, has been found using a different algorithm, as such an exact integration between the crossings is not possible in these cases: the time evolution of the system is approximated by a velocity Verlet algorithm for the $N$ particle forces, and collisions are implemented *after* each time step for all particle pairs which cross during the time step. The time step is chosen sufficiently short such that only crossings between particles which are nearest neighbours at the previous time step occur. This algorithm converges to the exact collisional dynamics when the time step goes to zero. When the perturbation arising from the inelastic collisions is switched off, the velocity update when particles cross is no longer performed and the algorithm becomes symplectic. As expected, one recovers a very accurate conservation of the total energy in this case. The initial conditions are chosen for most of our study are "rectangular waterbag", but as noted in the text, our results on the ordered states are essentially independent of them.

We have benchmarked our algorithm by comparing the results for the evolution of the sheet model ($\alpha = 1$) and the harmonic model ($\alpha = 2$) with those obtained for these cases with the event-driven algorithm (which provides an exact numerical of the equations of motion up to the round-off errors). We have found excellent agreement for the evolution of the macroscopic observables we have considered (notably the virial ratio, and the energy and velocity distributions), and the same ordered final states in all cases we checked (and, as in the other models, when we switch off the inelastic collisions these states persist over the very long times we simulate).

## II. EXPONENTS IN RANGE $1 < \alpha < 2$

We first consider this range where the force between particles vanishes when the distance goes to zero (and thus no regularisation at $r = 0$ is needed). We have studied various values, and find behaviours very similar to those for the cases $\alpha = 1$ and $\alpha = 2$. Just as is the case for the cases $\alpha = 1$ and $\alpha = 2$ when we compare them, the configurations at a given $N$ are not identical to those in either case: the number of circles at each $N$ is not the same.

Fig.1 shows the stable ordered configurations obtained for $N = 9, 10, ..., 18$ for $\alpha = 1.5$, and Fig.2 for the case $\alpha = 1.9$. For the first case we observe that from $N = 12$ upward the states start to differ e.g. relative to the model with $\alpha = 1$ in the number of particles on each circle: while for $\alpha = 1$ a second particle appears on the inner circle (of two) at $N = 12$, this transition now takes place at $N = 16$. For $\alpha = 1.9$ we also obtain ordered states, but again with slightly differing "critical" values for the transition in the numbers of particle per circle.

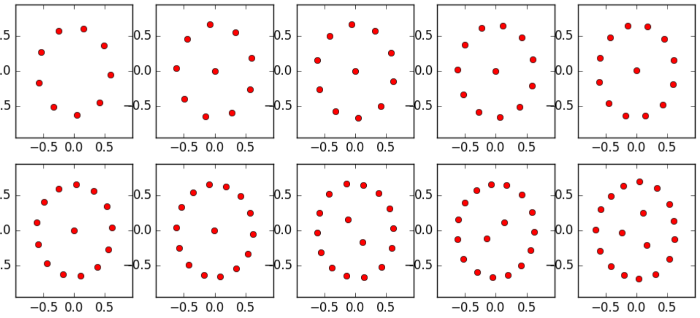

FIG. 1. Snapshots of the phase space of the system at different sizes $N = 9, 10, .., 18$ for a potential $v(r) = r^{1.5}$

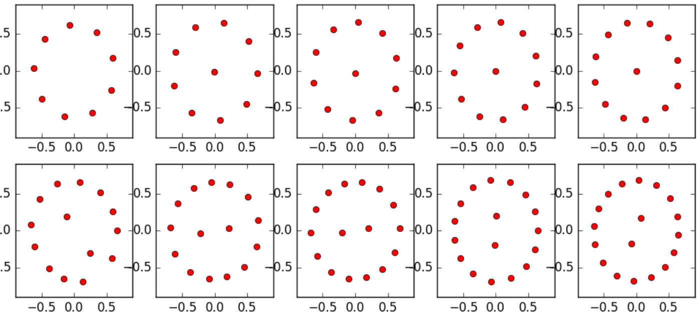

FIG. 2. Snapshots of the phase space of the system at different sizes $N = 9, 10, .., 18$ for a potential $v(r) = r^{1.9}$

## III. EXPONENTS IN RANGE $0 < \alpha < 1$

For $\alpha < 1$, the force diverges when the distance between particles goes to zero. As noted above we then regularise taking $v(r) = g[r^2 + \epsilon^2]^{\alpha/2}$, and $\epsilon \neq 0$. In practice we find that, provided $\epsilon$ is small compared to the interparticle separation, the evolution and ordered final states we again obtain are completely insensitive to the value of $\epsilon$, and indeed for the larger values of $\alpha$ we simulate we have obtained the same results even setting $\epsilon = 0$. This contrasts, as we report below, with the case $\alpha < 0$. As we discuss below, there is a simple explanation of this qualitative difference.

Fig. 3 and Fig. 4 show the stable ordered configurations obtained for the different values of $N$, for $\alpha = 0.8$ and $\alpha = 0.5$ respectively. We note that the ordered structure with multiple circles now appears for system sizes smaller than for the sheet model ($\alpha = 1$), and that the smaller is $\alpha$ the smaller is the corresponding system size.

## IV. EXPONENTS IN RANGE $-1 < \alpha < 0$

When we consider exponents $\alpha < 0$ we find that increasingly large values of $\epsilon$ are required to stabilise the results numerically (i.e. to conserve energy well and provide well converged results independent of the chosen time step). In practice we need to use, even for $\alpha = -0.2$, a value of $\epsilon$ at least of order one tenth of the the system size (and thus larger than the interparticle separation). When we do obtain such stability in this way, we again observe the emergence of the same ordered states. Fig .5 shows the results for the case $\alpha = -0.2$ and Fig .6 for the case $\alpha = -0.5$. We note that the trend towards the multiplication of the particles on the second inner circle at lower $N$ as we decrease $\alpha$ is further confirmed by these results.

This qualitative difference between the exponents $\alpha < 0$ and $1 > \alpha > 0$ arises, we believe, from the fact that this corresponds to the border between integrable and non-integrable pair forces (at large separations). As discussed in [2] (see also [3, 4]) this corresponds to a crucial difference for what concerns the dynamics of systems with power-law interactions in the large $N$ limit: if the pair force is integrable, the contribution to the net force from nearby particles

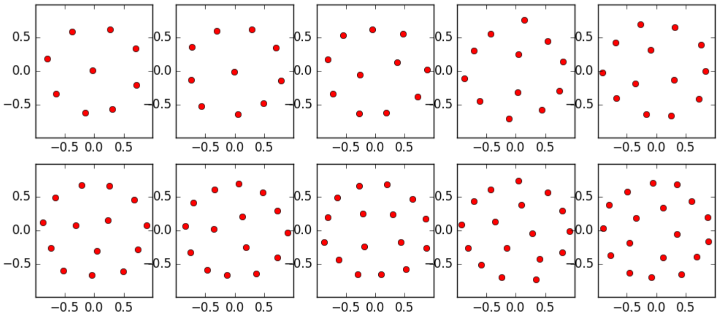

FIG. 3. Snapshots of the phase space of the system at different sizes $N = 9, 10, .., 18$ for a potential $v(r) = r^{0.8}$

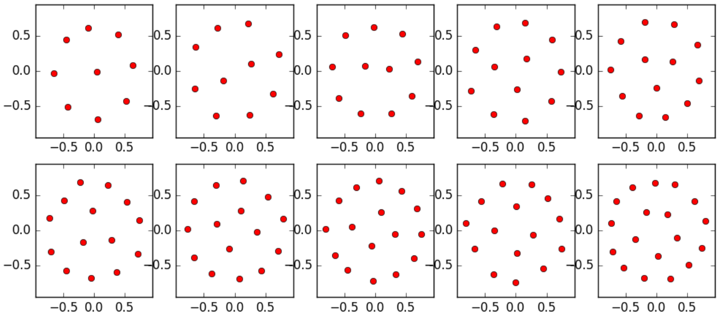

FIG. 4. Snapshots of the phase space of the system at different sizes $N = 9, 10, .., 18$ for a potential $v(r) = (r^2 + \epsilon)^{0.25}$ and $\epsilon = 0.01$

(at of order the mean-interparticle separation) dominates at sufficiently large $N$ over the bulk contribution unless a sufficiently large "softening" is introduced. It is the domination of the bulk (mean-field, in the infinite $N$ limit) contribution over the fluctuating short-range contribution to the force which leads to the characteristic behaviour of long-range systems, and in particular the establishment of QSS. At finite (and even not very large, as here) particle number, this difference means in practice that, without softening, the typical force acting on a particle is dominated by its nearest neighbour at a distance which increases as $\alpha$ decreases. If the force is smoothed at a separation large than this distance, the dynamics should become insensitive to it. Numerically the fact that no regularisation is apparently needed for values of $\alpha$ close to (but less than) unity can be attributed to the fact that the distance moved in a time-step is larger than this scale (but sufficiently small to simulate accurately the movement under the bulk force).

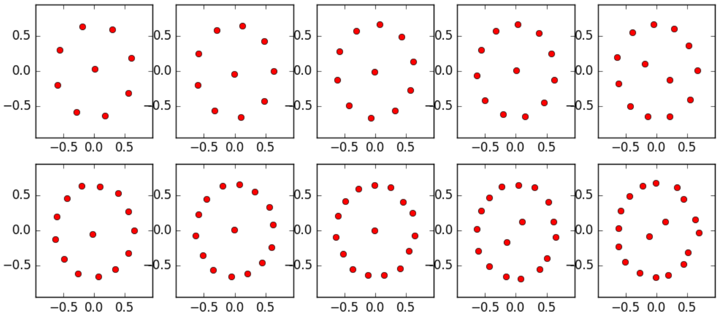


FIG. 5. Snapshots of the phase space of the system at different sizes $N = 9, 10, .., 18$ for a potential $v(r) = (r^2 + \epsilon)^{-0.1}$ and $\epsilon = 0.1$

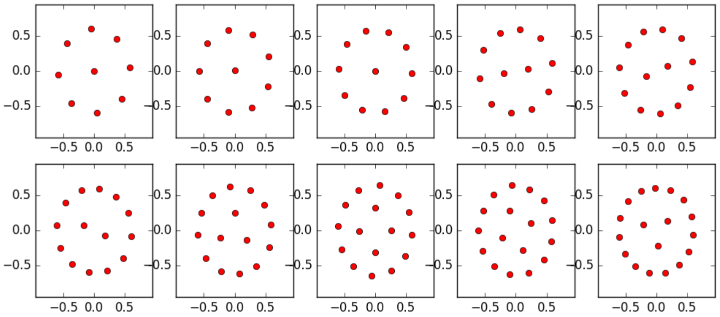


FIG. 6. Snapshots of the phase space of the system at different sizes $N = 9, 10, .., 18$ for a potential $v(r) = (r^2 + \epsilon)^{-0.25}$ and $\epsilon = 0.1$

## V. EXPONENTS $\alpha > 2$

We have explored also this range in which the potential grows faster than in the harmonic case. The results for the case $\alpha = 2.2$ and $\alpha = 2.5$ are shown in Fig. 7 and Fig. 8. As illustrated our finding is that, despite running for very long times, we observe only at low particle number the establishment of ordered states, and we never observe such a state with more than a single ring. Instead of the transition to a two ring state observed in all other cases, we find that the system remains in a configuration of a roughly circular, but more irregular, shape. A more complete study is required to confirm this finding, but it appears that for $\alpha > 2$ our stable ordered stable configurations only exist for small system sizes. The reason for this appears to be that, for $\alpha > 2$, that the particles of the system cannot produce together an approximately harmonic bulk potential which appears to be necessary in order to explain the characteristic synchronisation of the particles in the ordered states (with multiple circles).

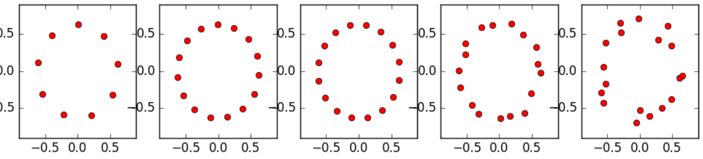


FIG. 7. Snapshots of the phase space of the system at different sizes $N = 9, 15, 16, 17, 18$ for a potential $v(r) = r^{2.2}$

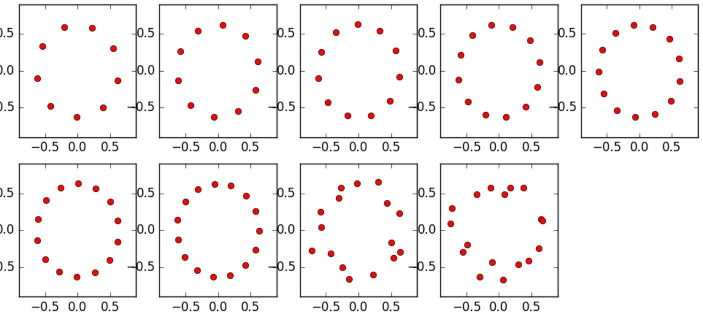


FIG. 8. Snapshots of the phase space of the system at different sizes $N = 9, 10, .., 17$ for a potential $v(r) = r^{2.5}$

## VI. HMF MODEL

To study the paradigmatic model HMF[5], we implement the appropriate modification of our algorithm for the power law (or softened power law) potentials. Exploring a range of values of $v_0$, we find that ordered configurations of the phase space again emerge robustly for any system size, but only provided the value of $v_0$ is sufficiently small (as the potential is now no longer scale invariant this has a meaning). This corresponds to a stationary state of very low energy and high magnetisation, with all the particles in a very small segment of the circle on which the model particles move, and thus to the limit in which the HMF potential is well approximated as harmonic. Fig 9 displays configurations of the system at different sizes $N = 9, 10, .., 18$.

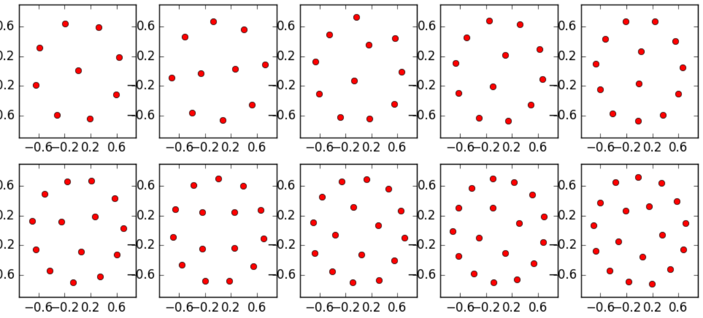


FIG. 9. Snapshots of the phase space of the system at different sizes $N = 9, 10, .., 18$ for the HMF model at small $v_0$ ($v_0 < 10^{-3}$ in the canonical natural units of model of the model)

In this case the apparent absence of these states again appears to be due to the fact that, beyond the region in which the interparticle potential is very well approximated as harmonic, the system is unable to produce a configuration leading to a bulk potential which is close to harmonic. Given the periodic structure of the HMF on a circle, this is evidently the case.

[1] M. Joyce and T. Worrakitpoonpon, J. Stat. Mech. **2010**, P10012 (2010).
[2] A. Gabrielli, M. Joyce, and B. Marcos, Phys. Rev. Lett. **105**, 210602 (2010).
[3] A. Gabrielli, M. Joyce, and J. Morand, Phys. Rev. E **90**, 062910 (2014).
[4] B. Marcos, A. Gabrielli, and M. Joyce, ArXiv e-prints (2017), arXiv:1701.01865 [cond-mat.stat-mech].
[5] A. Campa, T. Dauxois, and S. Ruffo, Phys. Rep. **480**, 57 (2009).
